# Supplementary material for: Anomalous light cones and valley optical selection rules of interlayer excitons in twisted heterobilayers
Source: arXiv:1504.01215 ancillary file (2015-10-16)
Supplement: Supplementary file 1 [file SupplementalMaterial.pdf]

# Supplemental Material for "Anomalous light cones and valley optical selection rules of interlayer excitons in twisted heterobilayers"

Hongyi Yu, Yong Wang, Qingjun Tong, Xiaodong Xu, Wang Yao

## Supplementary Note I. Interlayer electron-hole Coulomb interaction

We use $|e_{\tau',\mathbf{k}'}\rangle$ ($|h_{\tau,\mathbf{k}}\rangle$) to denote the electron (hole) Bloch state with wavefunction $\psi_{\tau',\mathbf{k}',\mathrm{c}}(\mathbf{r}_\mathrm{e}) = e^{i(\tau'\mathbf{K}'+\mathbf{k}')\cdot\mathbf{r}_\mathrm{e}} u_{\tau',\mathbf{k}',\mathrm{c}}(\mathbf{r}_\mathrm{e})$ ($\psi^*_{\tau,-\mathbf{k},\mathrm{v}}(\mathbf{r}_\mathrm{h}) = e^{-i(\tau\mathbf{K}-\mathbf{k})\cdot\mathbf{r}_\mathrm{h}} u^*_{\tau,-\mathbf{k},\mathrm{v}}(\mathbf{r}_\mathrm{h})$). The electron-hole interaction is dominated by the intravalley term of the direct Coulomb interaction: $V(\Delta\mathbf{k}',\Delta\mathbf{k})|e_{\tau',\mathbf{k}'+\Delta\mathbf{k}'}\rangle|h_{\tau,\mathbf{k}-\Delta\mathbf{k}}\rangle\langle h_{\tau,\mathbf{k}}|\langle e_{\tau',\mathbf{k}'}|$, where

$$V(\Delta\mathbf{k}',\Delta\mathbf{k}) \equiv \int d\mathbf{r}_\mathrm{e} d\mathbf{r}_\mathrm{h} \psi^*_{\tau',\mathbf{k}'+\Delta\mathbf{k}',c}(\mathbf{r}_\mathrm{e})\psi_{\tau,-\mathbf{k}+\Delta\mathbf{k},\mathrm{v}}(\mathbf{r}_\mathrm{h}) V(\mathbf{r}_\mathrm{e}-\mathbf{r}_\mathrm{h})\psi_{\tau',\mathbf{k}',c}(\mathbf{r}_\mathrm{e})\psi^*_{\tau,-\mathbf{k},\mathrm{v}}(\mathbf{r}_\mathrm{h})$$
$$= \sum_{\mathbf{G},\mathbf{G}'} \delta_{\mathbf{G}+\Delta\mathbf{k},\mathbf{G}'+\Delta\mathbf{k}'} V(\mathbf{G}+\Delta\mathbf{k})\eta'(\mathbf{G}')\eta(\mathbf{G}).$$

Here $V(\mathbf{r})$ is the Coulomb potential as a function of in-plane coordinates $\mathbf{r}$, $V(\mathbf{k}) \equiv \int d\mathbf{r} V(\mathbf{r}) e^{i\mathbf{k}\cdot\mathbf{r}}$, $\mathbf{G}'$ and $\mathbf{G}$ denote the reciprocal lattice vectors of the individual layers. $\eta'(\mathbf{G}') \equiv \int d\mathbf{r}_\mathrm{e} u^*_{\tau',\mathbf{k}'+\Delta\mathbf{k}',\mathrm{c}}(\mathbf{r}_\mathrm{e}) e^{i\mathbf{G}'\cdot\mathbf{r}_\mathrm{e}} u_{\tau',\mathbf{k}',\mathrm{c}}(\mathbf{r}_\mathrm{e}) = \langle e_{\tau',\mathbf{k}'+\Delta\mathbf{k}'}| e^{i(\mathbf{G}'+\Delta\mathbf{k}')\cdot\mathbf{r}_\mathrm{e}} |e_{\tau',\mathbf{k}'}\rangle$ and $\eta(\mathbf{G}) \equiv \int d\mathbf{r}_\mathrm{h} u^*_{\tau,-\mathbf{k},\mathrm{v}}(\mathbf{r}_\mathrm{h}) e^{-i\mathbf{G}\cdot\mathbf{r}_\mathrm{h}} u_{\tau,-\mathbf{k}+\Delta\mathbf{k},\mathrm{v}}(\mathbf{r}_\mathrm{h}) = \langle h_{\tau,\mathbf{k}-\Delta\mathbf{k}}| e^{-i(\mathbf{G}+\Delta\mathbf{k})\cdot\mathbf{r}_\mathrm{h}} |h_{\tau,\mathbf{k}}\rangle$. We are interested in low energy electrons and holes with $k, k', \Delta k, \Delta k' \ll K$. Therefore $\eta'(\mathbf{G}'=0) \approx \eta(\mathbf{G}=0) \approx 1$. While for $\mathbf{G}',\mathbf{G} \neq 0$, *ab initio* result shows $|\eta'(\mathbf{G}' \neq 0)| \lesssim 0.2$ and $|\eta(\mathbf{G} \neq 0)| \lesssim 0.1$. Besides, $V(\mathbf{G}+\Delta\mathbf{k}) \ll V(\Delta\mathbf{k})$ for $\mathbf{G} \neq 0$, therefore we only need to keep the $\mathbf{G}=\mathbf{G}'=0$ term:

$$V(\Delta\mathbf{k}',\Delta\mathbf{k}) \cong \delta_{\Delta\mathbf{k},\Delta\mathbf{k}'} V(\Delta\mathbf{k}). \quad \text{(S1)}$$

In the interlayer exciton formation, the effect of intervalley Coulomb scatterings are negligible as the corresponding $V(\mathbf{K})$ are weak and they are further suppressed by the large spin-orbit splitting. The electron-hole Coulomb exchange interaction is also negligible, as its strength is proportional to the electron-hole wave function overlap [1] which is largely suppressed for interlayer exciton.

The interlayer exciton is then the eigenstates of the Hamiltonian:

$$\hat{H}_X = \sum_{\tau',\mathbf{k}'} (E_{\tau',\mathbf{k}',\mathrm{c}} + \Delta_g)|e_{\tau',\mathbf{k}'}\rangle\langle e_{\tau',\mathbf{k}'}| + \sum_{\tau,\mathbf{k}} E_{\tau,\mathbf{k},\mathrm{v}} |h_{\tau,\mathbf{k}}\rangle\langle h_{\tau,\mathbf{k}}|$$
$$+ \sum_{\tau',\tau,\mathbf{k}',\mathbf{k},\Delta\mathbf{k}} V(\Delta\mathbf{k})|e_{\tau',\mathbf{k}'+\Delta\mathbf{k}}\rangle|h_{\tau,\mathbf{k}-\Delta\mathbf{k}}\rangle\langle h_{\tau,\mathbf{k}}|\langle e_{\tau',\mathbf{k}'}| \quad \text{(S2)}$$

Here $E_{\tau',\mathbf{k}',\mathrm{c}}$ and $E_{\tau,\mathbf{k},\mathrm{v}}$ are the electron and hole dispersions respectively, $\Delta_g$ is the band gap. Obviously the Coulomb interaction conserves $\mathbf{Q} \equiv \mathbf{k}'+\mathbf{k}$, the sum of the electron and hole momentums defined in the individual layers. The interlayer exciton wave function is [2,3]:

$$\left|X^{(0)}_{\tau'\tau,\mathbf{Q}}\right\rangle = \sum_{\Delta\mathbf{Q}} \Phi_I(\Delta\mathbf{Q}) \left|e_{\tau',\frac{m_\mathrm{e}}{M_0}\mathbf{Q}+\Delta\mathbf{Q}}\right\rangle \left|h_{\tau,\frac{m_\mathrm{h}}{M_0}\mathbf{Q}-\Delta\mathbf{Q}}\right\rangle$$
$$= e^{i\mathbf{Q}\cdot\left(\frac{m_\mathrm{e}}{M_0}\mathbf{r}_\mathrm{e}+\frac{m_\mathrm{h}}{M_0}\mathbf{r}_\mathrm{h}\right)} \sum_{\Delta\mathbf{Q}} \Phi_I(\Delta\mathbf{Q}) e^{i\Delta\mathbf{Q}\cdot(\mathbf{r}_\mathrm{e}-\mathbf{r}_\mathrm{h})} u_{\tau',\frac{m_\mathrm{e}}{M_0}\mathbf{Q}+\Delta\mathbf{Q}}(\mathbf{r}_\mathrm{e}) u^*_{\tau,-\frac{m_\mathrm{h}}{M_0}\mathbf{Q}+\Delta\mathbf{Q}}(\mathbf{r}_\mathrm{h}) \quad \text{(S3)}$$
$$\cong e^{i\mathbf{Q}\cdot\mathbf{R}_X} \Phi_I(\mathbf{r}_\mathrm{e}-\mathbf{r}_\mathrm{h}) u_{\tau',\frac{m_\mathrm{e}}{M_0}\mathbf{Q}}(\mathbf{r}_\mathrm{e}) u^*_{\tau,-\frac{m_\mathrm{h}}{M_0}\mathbf{Q}}(\mathbf{r}_\mathrm{h}).$$

Here $\mathbf{R}_X \equiv \frac{m_\mathrm{e}}{M_0}\mathbf{r}_\mathrm{e} + \frac{m_\mathrm{h}}{M_0}\mathbf{r}_\mathrm{h}$ is the exciton center-of-mass coordinate, $\Phi_I(\mathbf{r}) \equiv \sum_{\Delta\mathbf{Q}} \Phi_I(\Delta\mathbf{Q}) e^{i\Delta\mathbf{Q}\cdot\mathbf{r}}$ describes the real space electron-hole relative motion with $\Delta\mathbf{Q} \equiv (m_\mathrm{h}\mathbf{k}' - m_\mathrm{e}\mathbf{k})/M_0$. In the last step we used $u_{\tau',\frac{m_\mathrm{e}}{M_0}\mathbf{Q}+\Delta\mathbf{Q}} \approx u_{\tau',\frac{m_\mathrm{e}}{M_0}\mathbf{Q}}$ and $u^*_{\tau,-\frac{m_\mathrm{h}}{M_0}\mathbf{Q}+\Delta\mathbf{Q}} \approx u^*_{\tau,-\frac{m_\mathrm{h}}{M_0}\mathbf{Q}}$.

Theories and first principle calculations have shown that, while the binding energy is as large as hundreds of meV, the wavefunction for intralayer exciton in a monolayer is largely the Wannier type, with electron and hole both well localized in **k**-space at the nearly parabolic band edges in the $\pm\mathbf{K}$ valleys [4]. Moreover, the effective mass description is found to be rather successful in obtaining the binding energy and the Bohr radius [5]. So here we write $E_{\tau',\mathbf{k}',\mathrm{c}} = \frac{\hbar^2 k'^2}{2m_\mathrm{e}}$ and $E_{\tau,\mathbf{k},\mathrm{v}} = \frac{\hbar^2 k^2}{2m_\mathrm{h}}$, the corresponding energy of Eq. (S3) is $E_I(\mathbf{Q}) = \frac{\hbar^2 Q^2}{2M_0} + \Delta_g - E_b$.

In the heterobilayers, since the layer separation (~0.7 nm) is small compared to the intralayer exciton Bohr radius (one to several nm), it is expected that the interlayer Coulomb binding $E_b$ between the electron and hole in the two layers is not significantly reduced compared to the intralayer case. Moreover, there are experimental facts now on interlayer excitons. The optical measurement [6] combined with the STM measurement [7] implies the interlayer exciton binding energy to be in the order of a few hundred meV. Ref. [8] has also measured an interlayer exciton binding energy $E_b \sim 260\,\mathrm{meV}$, the same order of magnitude to that of intralayer exciton. Accordingly the interlayer exciton Bohr radius is also in the same order of magnitude (a few nm) to that of the intralayer exciton.

Considering the strong binding energy, here and below we restrict our discussion to interlayer exciton in the ground state of relative motion, as the excited states are expected to be several hundred meV higher.

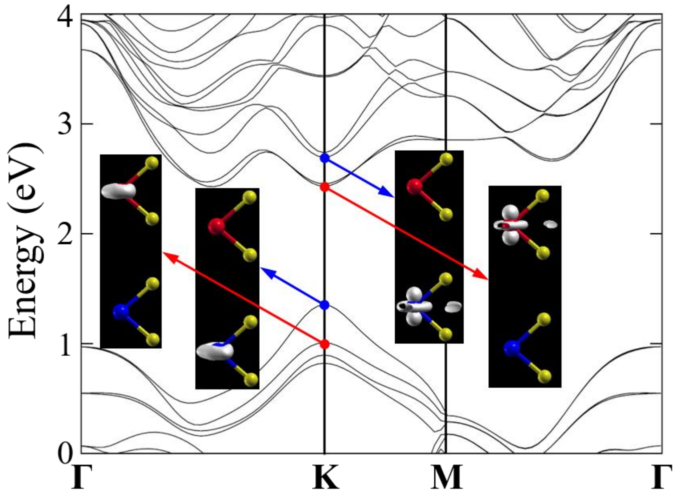


Supplementary Figure S1 | *Ab initio* band structure of lattice matching $MoSe_2/WSe_2$ heterobilayer with $\theta = 0$ and $\mathbf{r}_0 = 0$ (AA stacking). The insets show the conduction (valence) band edge wave functions at **K**, localized predominantly in the $MoSe_2$ ($WSe_2$) layer with very small interlayer hybridization, which shows that interlayer coupling is indeed weak compared to the band offsets. The *ab initio* calculations are performed with the fully relativistic pseudopotential in order to include the SOC, with other details the same as in Supplementary Note III.

**Supplementary Note II.  Interlayer hopping and interlayer dipole transition**

The heterobilayers can be characterized by a twisting angle $0^{\circ} \leq \theta \leq 60^{\circ}$, and a relative in-plane translation $\mathbf{r}_0$, with respect to a *reference stacking configuration*. Such a reference configuration can be defined as the one where the zigzag crystalline axes of the two layers coincide, and two metal atoms in the opposite layers horizontally overlap at in-plane coordinate $\mathbf{R}_0$. Any heterobilayer can then be obtained from this reference configuration through a rotation of $\theta$ around $\mathbf{R}_0$ followed by a translation of $\mathbf{r}_0$ of the upper layer. The two layers sharing the same *in-plane* coordinates, the positions of metal atoms in the upper (lower) layer can be written as $\mathbf{R}' = \mathbf{R}'_0 + l'\mathbf{a}'_1 + n'\mathbf{a}'_2$ ($\mathbf{R} = \mathbf{R}_0 + l\mathbf{a}_1 + n\mathbf{a}_2$) where $\mathbf{R}'_0 = \mathbf{R}_0 + \mathbf{r}_0$. $\mathbf{a}'_{1,2}$ ($\mathbf{a}_{1,2}$) are the unit lattice vectors in the upper (lower) layer, and $l$, $n$, $l'$, $n'$ are integers.

For each monolayer $MX_2$ (M=Mo/W, X=S/Se), the Bloch function of the band edge electron and hole at $\tau\mathbf{K}$ point ($\tau = \pm 1$ being the valley index) can be approximated as:

$$\psi_{\tau,\mathbf{k}=0,\mathrm{c}}(\mathbf{r}) = e^{i(\tau\mathbf{K})\cdot\mathbf{r}} u_{\tau,\mathbf{k}=0,\mathrm{c}}(\mathbf{r}) = \frac{1}{\sqrt{N}}\sum_{\mathbf{R}} e^{i\tau\mathbf{K}\cdot\mathbf{R}} D_{m=0,\mathbf{R}},$$
$$\psi_{\tau,\mathbf{k}=0,\mathrm{v}}(\mathbf{r}) = e^{i(\tau\mathbf{K})\cdot\mathbf{r}} u_{\tau,\mathbf{k}=0,\mathrm{v}}(\mathbf{r}) = \frac{1}{\sqrt{N}}\sum_{\mathbf{R}} e^{i\tau\mathbf{K}\cdot\mathbf{R}} D_{m=2\tau,\mathbf{R}}. \quad \text{(S4)}$$

Here $D_{m,\mathbf{R}} \equiv D_m(\mathbf{r}-\mathbf{R})$ is the tight-binding basis function, centered at M atom at position $\mathbf{R}$, whose majority component is $d_{m,\mathbf{R}} \equiv d_m(\mathbf{r}-\mathbf{R})$ orbital of the M atom. $m$ here is the magnetic quantum number of the M-d orbitals: $d_{m=0} \equiv d_{z^2}$ and $d_{m=\pm 2} \equiv \frac{d_{x^2-y^2} \pm i d_{xy}}{\sqrt{2}}$. $D_{m,\mathbf{R}}$ also has small components of $p_{\pm 1} \equiv \frac{p_x \pm i p_y}{\sqrt{2}}$ orbital of the six nearest neighbor X atoms (Supplementary Figure S2).

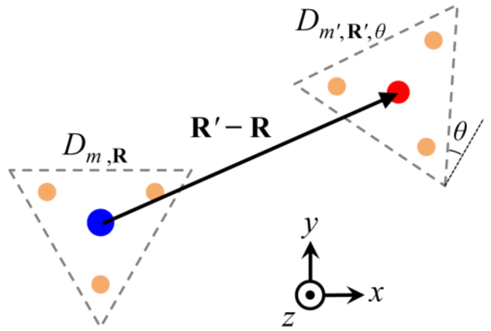


Supplementary Figure S2 | Schematic illustration of $D_{m,\mathbf{R}}$ ($D_{m',\mathbf{R}',\theta}$) centered at $\mathbf{R}$ ($\mathbf{R}'$) in the lower (upper) layer. $\theta$ is the twisting angle between the upper and lower layer. The red and blue dots denote the $d$ orbitals of the M atom (majority component), while the small orange dots denote the $p$ orbitals of the X atom (minority component).

The Bloch function at $\tau\mathbf{K} + \mathbf{k}$ ($k \ll K$) is given under the envelope function approximation:

$$\psi_{\tau,\mathbf{k},\mathrm{c(v)}}(\mathbf{r}) \cong e^{i(\tau\mathbf{K}+\mathbf{k})\cdot\mathbf{r}} u_{\tau,\mathbf{k}=0,\mathrm{c(v)}}(\mathbf{r}) = \frac{1}{\sqrt{N}}\sum_{\mathbf{R}} e^{i(\tau\mathbf{K}\cdot\mathbf{R}+\mathbf{k}\cdot\mathbf{r})} D_{m,\mathbf{R}} \cong \frac{1}{\sqrt{N}}\sum_{\mathbf{R}} e^{i(\tau\mathbf{K}+\mathbf{k})\cdot\mathbf{R}} D_{m,\mathbf{R}}.$$

where the last step ($e^{i\mathbf{k}\cdot(\mathbf{r}-\mathbf{R})} D_{m,\mathbf{R}} \cong D_{m,\mathbf{R}}$) is from the fact that $k \ll K$ and $D_{m,\mathbf{R}}$ is well localized around $\mathbf{R}$.

Treating $\hat{H}_{\mathrm{T}}$ as a perturbation, the interlayer exciton eigenstate is then

$$\left|X^{(1)}_{\tau'\tau,\mathbf{Q}}\right\rangle = \left|X^{(0)}_{\tau'\tau,\mathbf{Q}}\right\rangle + \sum_{\mathbf{q}} \frac{\left\langle X_{\tau',\mathbf{q}}\middle|\hat{H}_{\mathrm{T}}\middle|X^{(0)}_{\tau'\tau,\mathbf{Q}}\right\rangle}{E_I(\mathbf{Q})-E_{\mathrm{M}}}\left|X_{\tau',\mathbf{q}}\right\rangle + \sum_{\mathbf{q}} \frac{\left\langle X_{\tau,\mathbf{q}}\middle|\hat{H}_{\mathrm{T}}\middle|X^{(0)}_{\tau'\tau,\mathbf{Q}}\right\rangle}{E_I(\mathbf{Q})-E_{\mathrm{W}}}\left|X_{\tau,\mathbf{q}}\right\rangle,$$

where $\left|X_{\tau',\mathbf{q}}\right\rangle$ ($\left|X_{\tau,\mathbf{q}}\right\rangle$) is the intralayer exciton with the center-of-mass wave vector $\mathbf{q}$ defined in a monolayer $MoX_2$ ($WX_2$).

The interlayer exciton transition dipole is

$$\boldsymbol{\mathcal{D}}_{\tau'\tau,\mathbf{Q}} = \left\langle 0\middle|\hat{\mathbf{D}}\middle|X^{(0)}_{\tau'\tau,\mathbf{Q}}\right\rangle + \frac{\left\langle X_{\tau'}\middle|\hat{H}_{\mathrm{T}}\middle|X^{(0)}_{\tau'\tau,\mathbf{Q}}\right\rangle}{E_I(\mathbf{Q})-E_{\mathrm{M}}}\left\langle 0\middle|\hat{\mathbf{D}}\middle|X_{\tau'}\right\rangle + \frac{\left\langle X_{\tau}\middle|\hat{H}_{\mathrm{T}}\middle|X^{(0)}_{\tau'\tau,\mathbf{Q}}\right\rangle}{E_I(\mathbf{Q})-E_{\mathrm{W}}}\left\langle 0\middle|\hat{\mathbf{D}}\middle|X_{\tau}\right\rangle. \tag{S5}$$

On the right hand side the first term is from the *interlayer transition dipole* between Bloch function $\psi_{\tau',\mathbf{k}',c}$ defined in $MoX_2$ layer and the Bloch function $\psi_{\tau,-\mathbf{k},v}$ in $WX_2$ which is small because of the spatial separation. The second and third terms describe respectively the light coupling mediated by bright intralayer exciton $X_{\tau'} \equiv X_{\tau',\mathbf{q}=0}$ in $MoX_2$ layer through hole interlayer hopping, and $X_\tau \equiv X_{\tau,\mathbf{q}=0}$ in $WX_2$ through electron hopping.

The intralayer exciton transition dipole $\left\langle 0\middle|\hat{\mathbf{D}}\middle|X_\tau\right\rangle = D\mathbf{e}_\tau$ [1], where the unit polarization vector $\mathbf{e}_\pm \equiv \frac{\mathrm{x}\pm i\mathrm{y}}{\sqrt{2}}$ reflects the valley optical selection rule, and the dipole strength $D$ is [3]

$$D = \sum_{\Delta\mathbf{Q}} \Phi(\Delta\mathbf{Q})\big(\mathbf{d}_{\mathrm{vc},\tau}(\Delta\mathbf{Q})\cdot\mathbf{e}_\tau\big),$$

Here $\mathbf{d}_{\mathrm{vc},\tau}(\Delta\mathbf{Q}) \equiv \left\langle\psi_{\tau,\Delta\mathbf{Q},\mathrm{v}}\middle|\hat{\mathbf{D}}\middle|\psi_{\tau,\Delta\mathbf{Q},\mathrm{c}}\right\rangle$ is the band-to-band transition dipole in a monolayer, and $\Phi$ is the intralayer exciton wavefunction in **k**-space ($\left|X_\pm\right\rangle = \sum_{\Delta\mathbf{Q}}\Phi(\Delta\mathbf{Q})\left|e_{\pm,\Delta\mathbf{Q}}\right\rangle\left|h_{\pm,-\Delta\mathbf{Q}}\right\rangle$). $\Phi(\Delta\mathbf{Q})$ is distributed around $\pm\mathbf{K}$ in a range $\Delta Q \lesssim 1/a_B$ [4], over which the **k**-dependence of $\mathbf{d}_{\mathrm{vc},\tau}$ is weak. Replace $\mathbf{d}_{\mathrm{vc},\tau}(\Delta\mathbf{Q})$ by its value at $\tau\mathbf{K}$, then $D \approx \Phi(\mathbf{r}=0)\big(\mathbf{d}_{\mathrm{vc},\tau}\cdot\mathbf{e}_\tau\big)$, where $\Phi(\mathbf{r}=0) \equiv \sum_{\Delta\mathbf{Q}}\Phi(\Delta\mathbf{Q}) \sim \sqrt{A}/a_B$. $A$ is the area of the box-normalization which goes away in measurable quantities such as the vacuum Rabi splitting of exciton in a planar cavity: $2DE_c \approx 2\sqrt{\frac{\hbar\omega_c}{\varepsilon L a_B^2}}\left|\mathbf{d}_{\mathrm{vc},\tau}\cdot\mathbf{e}_\tau\right|$ (where $L$ is the cavity length, and $E_c \propto 1/\sqrt{A}$ the average electric field of a cavity photon) [9]. We can use this Rabi splitting to characterize the exciton dipole strength, which is measured in Ref. [9] to be 20 meV for monolayer MoSe2 in a cavity with $L = 2.3\ \mu m$, about one order of magnitude stronger than that in GaAs quantum well, and the enhancement here is due to the small Bohr radius $a_B$ in TMDs.

Using the interlayer exciton wave function Eq. (S3), we can write [3]

$$\left\langle 0\middle|\hat{\mathbf{D}}\middle|X^{(0)}_{\tau'\tau,\mathbf{Q}}\right\rangle \approx \Phi(\mathbf{r}=0)\left\langle\psi_{\tau,-\mathbf{k},\mathrm{v}}\middle|\hat{\mathbf{D}}\middle|\psi_{\tau',\mathbf{k}',\mathrm{c}}\right\rangle$$

$$\left\langle X_{\tau'}\middle|\hat{H}_{\mathrm{T}}\middle|X^{(0)}_{\tau'\tau,\mathbf{Q}}\right\rangle \approx f'(\mathbf{Q})\left\langle\psi_{\tau,-\mathbf{k},\mathrm{v}}\middle|\hat{H}_{\mathrm{T}}\middle|\psi_{\tau',\mathbf{k}',\mathrm{v}}\right\rangle,$$

$$\left\langle X_{\tau}\middle|\hat{H}_{\mathrm{T}}\middle|X^{(0)}_{\tau'\tau,\mathbf{Q}}\right\rangle \approx f(\mathbf{Q})\left\langle\psi_{\tau,-\mathbf{k},\mathrm{c}}\middle|\hat{H}_{\mathrm{T}}\middle|\psi_{\tau',\mathbf{k}',\mathrm{c}}\right\rangle,$$

For $Q \lesssim 0.1K$, $f(\mathbf{Q}) \equiv \sum_{\Delta\mathbf{Q}}\Phi^*(\Delta\mathbf{Q})\Phi_I\left(\Delta\mathbf{Q}+\frac{m_{\mathrm{h}}}{M_0}\mathbf{Q}\right) \sim 1$, $f'(\mathbf{Q}) \equiv \sum_{\Delta\mathbf{Q}}\Phi'^*(\Delta\mathbf{Q})\Phi_I\left(\Delta\mathbf{Q}-\frac{m_{\mathrm{e}}}{M_0}\mathbf{Q}\right) \sim 1$.

Below we analyze the interlayer hopping and interlayer dipole transition matrix elements based on the two-center approximation where the hopping and dipole integral between two sites

depends only on the in-plane projection of their separation [10].

The interlayer hopping and transition dipole matrix element between the Bloch states in the upper (with the primed indices) and lower (with unprimed indices) layers is

$$\langle \psi_{\tau,-\mathbf{k},\mathrm{c(v)}} | \hat{H}_\mathrm{T} | \psi_{\tau',\mathbf{k}',\mathrm{c(v)}} \rangle = \sum_{\mathbf{R},\mathbf{R}'} \frac{e^{i(\tau'\mathbf{K}'+\mathbf{k}')\cdot\mathbf{R}'-i(\tau\mathbf{K}-\mathbf{k})\cdot\mathbf{R}}}{\sqrt{NN'}} \langle D_{m,\mathbf{R}} | \hat{H}_\mathrm{T} | D_{m',\mathbf{R}',\theta} \rangle,$$
$$\langle \psi_{\tau,-\mathbf{k},\mathrm{v}} | \hat{\mathbf{D}} | \psi_{\tau',\mathbf{k}',\mathrm{c}} \rangle = \sum_{\mathbf{R},\mathbf{R}'} \frac{e^{i(\tau'\mathbf{K}'+\mathbf{k}')\cdot\mathbf{R}'-i(\tau\mathbf{K}-\mathbf{k})\cdot\mathbf{R}}}{\sqrt{NN'}} \langle D_{m=2\tau,\mathbf{R}} | \hat{\mathbf{D}} | D_{m'=0,\mathbf{R}',\theta} \rangle. \tag{S6}$$

$D_{m',\mathbf{R}',\theta}$ with the subscript $\theta$ stands for the rotation of $D_{m',\mathbf{R}'}$ by $\theta$ angle (see Supplementary Figure S2). $\langle D_{m,\mathbf{R}} | \hat{H}_\mathrm{T} | D_{m',\mathbf{R}',\theta} \rangle$ ($\langle D_{m,\mathbf{R}} | \hat{\mathbf{D}} | D_{m',\mathbf{R}',\theta} \rangle$) is the hopping (transition dipole) integral between the localized orbital $D_{m',\mathbf{R}',\theta}$ at position $\mathbf{R}'$ in the upper layer and $D_{m,\mathbf{R}}$ at $\mathbf{R}$ in the lower layer, which depends only on $\mathbf{R}'-\mathbf{R}$ within the two-center approximation [10]. By Fourier transforms $t_{m'}^{m}(\mathbf{q},\theta) \equiv \frac{1}{\sqrt{\Omega'\Omega}} \int \langle D_{m,\mathbf{R}} | \hat{H}_\mathrm{T} | D_{m',\mathbf{R}',\theta} \rangle e^{i\mathbf{q}\cdot(\mathbf{R}'-\mathbf{R})} d[\mathbf{R}'-\mathbf{R}]$ and $\mathbf{D}_0^{2\tau}(\mathbf{q},\theta) \equiv \frac{1}{\sqrt{\Omega'\Omega}} \int \langle D_{m=2\tau,\mathbf{R}} | \hat{\mathbf{D}} | D_{m'=0,\mathbf{R}',\theta} \rangle e^{i\mathbf{q}\cdot(\mathbf{R}'-\mathbf{R})} d[\mathbf{R}'-\mathbf{R}]$, we have

$$\langle D_{m,\mathbf{R}} | \hat{H}_\mathrm{T} | D_{m',\mathbf{R}',\theta} \rangle = \frac{1}{\sqrt{NN'}} \sum_{\mathbf{q}} t_{m'}^{m}(\mathbf{q},\theta) e^{-i\mathbf{q}\cdot(\mathbf{R}'-\mathbf{R})},$$
$$\langle D_{m=2\tau,\mathbf{R}} | \hat{\mathbf{D}} | D_{m'=0,\mathbf{R}',\theta} \rangle = \frac{1}{\sqrt{NN'}} \sum_{\mathbf{q}} \mathbf{D}_0^{2\tau}(\mathbf{q},\theta) e^{-i\mathbf{q}\cdot(\mathbf{R}'-\mathbf{R})}, \tag{S7}$$

similar to the formulation of interlayer hopping matrix element in twisted bilayer graphene in two-center approximation [10]. Here $N'$ ($N$) is the number of unit cells in the upper (lower) layer, and $\Omega'$ ($\Omega$) is the area of the unit cell. Then

$$\begin{aligned}
\langle \psi_{\tau,-\mathbf{k},\mathrm{c(v)}} | \hat{H}_\mathrm{T} | \psi_{\tau',\mathbf{k}',\mathrm{c(v)}} \rangle &= \sum_{\mathbf{R},\mathbf{R}'} \frac{e^{i(\tau'\mathbf{K}'+\mathbf{k}')\cdot\mathbf{R}'-i(\tau\mathbf{K}-\mathbf{k})\cdot\mathbf{R}}}{N'N} \sum_{\mathbf{q}} t_{m'}^{m}(\mathbf{q},\theta) e^{-i\mathbf{q}\cdot(\mathbf{R}'-\mathbf{R})} \\
&= \sum_{\mathbf{G}',\mathbf{G},\mathbf{q}} \delta_{\tau'\mathbf{K}'+\mathbf{k}'-\mathbf{q},\mathbf{G}'} \delta_{\tau\mathbf{K}-\mathbf{k}-\mathbf{q},\mathbf{G}} t_{m'}^{m}(\mathbf{q},\theta) e^{-i\mathbf{G}\cdot\mathbf{R}_0+i\mathbf{G}'\cdot\mathbf{R}_0'} \\
&= \sum_{\mathbf{G}',\mathbf{G}} \delta_{\tau'\mathbf{K}'+\mathbf{k}'+\mathbf{G}',\tau\mathbf{K}-\mathbf{k}+\mathbf{G}} t_{m'}^{m}(\tau\mathbf{K}-\mathbf{k}+\mathbf{G},\theta) e^{i\mathbf{G}\cdot\mathbf{R}_0-i\mathbf{G}'\cdot\mathbf{R}_0'} \\
&\approx \sum_{\mathbf{G}',\mathbf{G}} \delta_{\tau'\mathbf{K}'+\mathbf{k}'+\mathbf{G}',\tau\mathbf{K}-\mathbf{k}+\mathbf{G}} t_{m'}^{m}(\tau\mathbf{K}+\mathbf{G},\theta) e^{i\mathbf{G}\cdot\mathbf{R}_0-i\mathbf{G}'\cdot\mathbf{R}_0'}, \\
\langle \psi_{\tau,-\mathbf{k},\mathrm{v}} | \hat{\mathbf{D}} | \psi_{\tau',\mathbf{k}',\mathrm{c}} \rangle &\approx \sum_{\mathbf{G}',\mathbf{G}} \delta_{\tau'\mathbf{K}'+\mathbf{k}'+\mathbf{G}',\tau\mathbf{K}-\mathbf{k}+\mathbf{G}} \mathbf{D}_0^{2\tau}(\tau\mathbf{K}+\mathbf{G},\theta) e^{i\mathbf{G}\cdot\mathbf{R}_0-i\mathbf{G}'\cdot\mathbf{R}_0'}.
\end{aligned} \tag{S8}$$

Here $\mathbf{G}'$ ($\mathbf{G}$) is the reciprocal lattice vectors of the upper (lower) layer. We have used $t_{m'}^{m}(\tau\mathbf{K}-\mathbf{k}+\mathbf{G},\theta) \approx t_{m'}^{m}(\tau\mathbf{K}+\mathbf{G},\theta)$ and $\mathbf{D}_0^{2\tau}(\tau\mathbf{K}-\mathbf{k}+\mathbf{G},\theta) \approx \mathbf{D}_0^{2\tau}(\tau\mathbf{K}+\mathbf{G},\theta)$ since $k \ll K$. We also expect $t_{m'}^{m}(\mathbf{q},\theta)$ and $\mathbf{D}_0^{2\tau}(\mathbf{q},\theta)$ to decay fast with the increase of $|\mathbf{q}|$, as the integrals $\langle D_{m,\mathbf{R}} | \hat{H}_\mathrm{T} | D_{m',\mathbf{R}',\theta} \rangle$ and $\langle D_{m=2\tau,\mathbf{R}} | \hat{\mathbf{D}} | D_{m'=0,\mathbf{R}',\theta} \rangle$ are generally smooth functions of $\mathbf{R}'-\mathbf{R}$.

Note that in Eq. (S8), $\mathbf{R}_0$, $\mathbf{R}_0'$ appear in the phase factor $e^{i\mathbf{G}\cdot\mathbf{R}_0-i\mathbf{G}'\cdot\mathbf{R}_0'}$ only. These are the positions of the reference W and Mo atoms, from which we define the relative layer translation $\mathbf{r}_0 = \mathbf{R}_0' - \mathbf{R}_0$. Although the value of $\mathbf{r}_0$ depends on the choice of the pair of reference atoms, the

interlayer hopping and transition dipole matrix elements are not affected by this uncertainty at all. This is obvious from the fact that $e^{i\mathbf{G}\cdot\mathbf{R}_0-i\mathbf{G}'\cdot\mathbf{R}'_0}$ is unchanged when $\mathbf{R}'_0$ ($\mathbf{R}_0$) is replaced by $\mathbf{R}'=\mathbf{R}'_0+l'\mathbf{a}'_1+n'\mathbf{a}'_2$ ($\mathbf{R}=\mathbf{R}_0+l\mathbf{a}_1+n\mathbf{a}_2$), the coordinate of any other metal atom in the upper (lower) layer, since $\mathbf{G}'\cdot(l'\mathbf{a}'_1+n'\mathbf{a}'_2)$ and $\mathbf{G}\cdot(l\mathbf{a}_1+n\mathbf{a}_2)$ are integer times of $2\pi$. In another word, heterbilayer configurations with $\mathbf{r}_0$ values differ only by $(l'\mathbf{a}'_1+n'\mathbf{a}'_2)-(l\mathbf{a}_1+n\mathbf{a}_2)$ are *equivalent.*

For lattice matching heterobilayers at $\theta=0^\circ$ or $60^\circ$, $(l'\mathbf{a}'_1+n'\mathbf{a}'_2)-(l\mathbf{a}_1+n\mathbf{a}_2)$ have the same set of values as $l'\mathbf{a}'_1+n'\mathbf{a}'_2$ (and $l\mathbf{a}_1+n\mathbf{a}_2$). In such case we can restrict $\mathbf{r}_0$ to take value within the unit cell of the lower layer (c.f. Figure 3 of main text), and heterobilayer configurations are uniquely specified by $\mathbf{r}_0$.

Let $\tau'\boldsymbol{\kappa}'\equiv\tau'\mathbf{K}'+\mathbf{G}'$ ($\tau\boldsymbol{\kappa}\equiv\tau\mathbf{K}+\mathbf{G}$), and using the fact $\delta_{\tau'\boldsymbol{\kappa}'+\mathbf{k}',\tau\boldsymbol{\kappa}-\mathbf{k}}e^{i\mathbf{G}\cdot\mathbf{R}_0-i\mathbf{G}'\cdot\mathbf{R}'_0}=\delta_{\mathbf{k}+\mathbf{k}',\tau\boldsymbol{\kappa}-\tau'\boldsymbol{\kappa}'}e^{-i\mathbf{G}\cdot\mathbf{r}_0}e^{i(\tau'\mathbf{K}'+\mathbf{k}'-\tau\mathbf{K}+\mathbf{k})\cdot\mathbf{R}'_0}$, Eq. (S8) becomes

$$\begin{aligned}\langle\psi_{\tau,-\mathbf{k},\mathrm{c(v)}}|\hat{H}_\mathrm{T}|\psi_{\tau',\mathbf{k}',\mathrm{c(v)}}\rangle&=e^{i(\tau'\mathbf{K}'+\mathbf{k}'-\tau\mathbf{K}+\mathbf{k})\cdot\mathbf{R}'_0}\left(e^{i\tau\mathbf{K}\cdot\mathbf{r}_0}\sum_{\boldsymbol{\kappa}',\boldsymbol{\kappa}}\delta_{\mathbf{Q},\tau\boldsymbol{\kappa}-\tau'\boldsymbol{\kappa}'}t^m_{m'}(\tau\boldsymbol{\kappa},\theta)e^{-i\tau\boldsymbol{\kappa}\cdot\mathbf{r}_0}\right),\\ \langle\psi_{\tau,-\mathbf{k},\mathrm{v}}|\hat{\mathbf{D}}|\psi_{\tau',\mathbf{k}',\mathrm{c}}\rangle&=e^{i(\tau'\mathbf{K}'+\mathbf{k}'-\tau\mathbf{K}+\mathbf{k})\cdot\mathbf{R}'_0}\left(e^{i\tau\mathbf{K}\cdot\mathbf{r}_0}\sum_{\boldsymbol{\kappa}',\boldsymbol{\kappa}}\delta_{\mathbf{Q},\tau\boldsymbol{\kappa}-\tau'\boldsymbol{\kappa}'}\mathbf{D}^{2\tau}_0(\tau\boldsymbol{\kappa},\theta)e^{-i\tau\boldsymbol{\kappa}\cdot\mathbf{r}_0}\right).\end{aligned}\tag{S9}$$

Clearly, different choices of $\mathbf{R}'_0$ correspond to different gauges, which do not affect measurable physical quantities. To simplify the expression we choose the gauge $\mathbf{R}'_0=0$. We also drop the $e^{i\tau\mathbf{K}\cdot\mathbf{r}_0}$ factor as it is a fixed constant for an exciton with the certain valley index and under the given heterobilayer configuration. The total transition dipole can be written as $\boldsymbol{\mathcal{D}}_{\tau'\tau,\mathbf{Q}}=\sum_{\boldsymbol{\kappa}',\boldsymbol{\kappa}}\delta_{\mathbf{Q},\tau\boldsymbol{\kappa}-\tau'\boldsymbol{\kappa}'}\boldsymbol{\mathcal{D}}_{\tau'\tau}(\tau\boldsymbol{\kappa},\theta)e^{-i\tau\boldsymbol{\kappa}\cdot\mathbf{r}_0}$, with

$$\begin{aligned}\boldsymbol{\mathcal{D}}_{\tau'\tau}(\tau\boldsymbol{\kappa},\theta)\equiv{}&\Phi_I(\mathbf{r}=0)\mathbf{D}^{2\tau}_0(\tau\boldsymbol{\kappa},\theta)+f'(\mathbf{Q})\frac{\langle0|\hat{\mathbf{D}}|X_{\tau'}\rangle}{E_I(\mathbf{Q})-E_\mathrm{M}}t^{2\tau}_{2\tau'}(\tau\boldsymbol{\kappa},\theta)\\&+f(\mathbf{Q})\frac{\langle0|\hat{\mathbf{D}}|X_\tau\rangle}{E_I(\mathbf{Q})-E_\mathrm{W}}t^0_0(\tau\boldsymbol{\kappa},\theta).\end{aligned}$$

Below we analyze the properties of $\boldsymbol{\mathcal{D}}_{\tau'\tau}(\tau\boldsymbol{\kappa},\theta)$ based on the symmetry of the monolayer lattice.

**(1) $\hat{C}_3$-rotational symmetry**

$\hat{C}_3$ denotes the in-plane $\frac{2}{3}\pi$-rotation about the origin. From the rotational symmetry of the atomic orbitals, $\langle D_{m,\hat{C}_3\mathbf{R}}|\hat{H}_\mathrm{T}|D_{m',\hat{C}_3\mathbf{R}',\theta}\rangle=e^{i\frac{2}{3}(m-m')\pi}\langle D_{m,\mathbf{R}}|\hat{H}_\mathrm{T}|D_{m',\mathbf{R}',\theta}\rangle$, and $\langle D_{m=2\tau,\hat{C}_3\mathbf{R}}|(\mathbf{e}_n\cdot\hat{\mathbf{D}})|D_{m'=0,\hat{C}_3\mathbf{R}',\theta}\rangle=e^{i\frac{2}{3}(\tau-n)\pi}\langle D_{m=2\tau,\mathbf{R}}|(\mathbf{e}_n\cdot\hat{\mathbf{D}})|D_{m'=0,\mathbf{R}',\theta}\rangle$. So

$$\begin{aligned}t^m_{m'}(\mathbf{q},\theta)&\equiv\frac{1}{\sqrt{\Omega'\Omega}}\int\langle D_{m,\mathbf{R}}|\hat{H}_\mathrm{T}|D_{m',\mathbf{R}',\theta}\rangle e^{i\mathbf{q}\cdot(\mathbf{R}'-\mathbf{R})}d[\mathbf{R}'-\mathbf{R}]\\&=\frac{e^{-i\frac{2}{3}(m-m')\pi}}{\sqrt{\Omega'\Omega}}\int\langle D_{m,\hat{C}_3\mathbf{R}}|\hat{H}_\mathrm{T}|D_{m',\hat{C}_3\mathbf{R}',\theta}\rangle e^{i\hat{C}_{3\mathbf{k}}\mathbf{q}\cdot\hat{C}_3(\mathbf{R}'-\mathbf{R})}d[\mathbf{R}'-\mathbf{R}]\\&=e^{-i\frac{2}{3}(m-m')\pi}t^m_{m'}(\hat{C}_{3\mathbf{k}}\mathbf{q},\theta),\end{aligned}$$

$$\mathbf{e}_n \cdot \mathbf{D}_0^{2\tau}(\mathbf{q},\theta) \equiv \frac{1}{\sqrt{\Omega'\Omega}}\int \left\langle D_{m=2\tau,\mathbf{R}}\middle|\left(\mathbf{e}_n \cdot \widehat{\mathbf{D}}\right)\middle|D_{m'=0,\mathbf{R}',\theta}\right\rangle e^{i\hat{C}_{3\mathbf{k}}\mathbf{q}\cdot\hat{C}_3(\mathbf{R}'-\mathbf{R})} d[\mathbf{R}'-\mathbf{R}]$$

$$= e^{-i\frac{2}{3}(\tau-n)\pi}\mathbf{e}_n \cdot \mathbf{D}_0^{2\tau}\left(\hat{C}_{3\mathbf{k}}\mathbf{q},\theta\right).$$

Therefore $t_{m'}^{m}\left(\hat{C}_{3\mathbf{k}}\mathbf{q},\theta\right) = t_{m'}^{m}(\mathbf{q},\theta)e^{i\frac{2}{3}(m-m')\pi}$, and $\mathbf{e}_n \cdot \mathbf{D}_0^{2\tau}\left(\hat{C}_{3\mathbf{k}}\mathbf{q},\theta\right) = e^{i\frac{2}{3}(\tau-n)\pi}\mathbf{e}_n \cdot \mathbf{D}_0^{2\tau}(\mathbf{q},\theta)$. We find the three components of $\boldsymbol{\mathcal{D}}_{\tau'\tau}(\tau\boldsymbol{\kappa},\theta)$ are:

$$\begin{pmatrix}\tau' = +1\\ \tau = +1\end{pmatrix}\begin{cases}\mathbf{e}_+ \cdot \boldsymbol{\mathcal{D}}_{++}(\boldsymbol{\kappa},\theta) = \Phi_I(0)\mathbf{e}_+ \cdot \mathbf{D}_0^{+2}(\boldsymbol{\kappa},\theta) + \dfrac{t_{+2}^{+2}(\boldsymbol{\kappa},\theta)}{E_I - E_\mathrm{M}}D' + \dfrac{t_0^{0}(\boldsymbol{\kappa},\theta)}{E_I - E_\mathrm{W}}D,\\ \mathbf{e}_- \cdot \boldsymbol{\mathcal{D}}_{++}(\boldsymbol{\kappa},\theta) = \Phi_I(0)\mathbf{e}_- \cdot \mathbf{D}_0^{+2}(\boldsymbol{\kappa},\theta),\\ \mathbf{e}_0 \cdot \boldsymbol{\mathcal{D}}_{++}(\boldsymbol{\kappa},\theta) = \Phi_I(0)\mathbf{e}_0 \cdot \mathbf{D}_0^{+2}(\boldsymbol{\kappa},\theta).\end{cases}$$

$$\begin{pmatrix}\tau' = -1\\ \tau = +1\end{pmatrix}\begin{cases}\mathbf{e}_+ \cdot \boldsymbol{\mathcal{D}}_{-+}(\boldsymbol{\kappa},\theta) = \Phi_I(0)\mathbf{e}_+ \cdot \mathbf{D}_0^{+2}(\boldsymbol{\kappa},\theta) + \dfrac{t_0^{0}(\boldsymbol{\kappa},\theta)}{E_I - E_\mathrm{W}}D,\\ \mathbf{e}_- \cdot \boldsymbol{\mathcal{D}}_{-+}(\boldsymbol{\kappa},\theta) = \Phi_I(0)\mathbf{e}_- \cdot \mathbf{D}_0^{+2}(\boldsymbol{\kappa},\theta) + \dfrac{t_{-2}^{+2}(\boldsymbol{\kappa},\theta)}{E_I - E_\mathrm{M}}D',\\ \mathbf{e}_0 \cdot \boldsymbol{\mathcal{D}}_{-+}(\boldsymbol{\kappa},\theta) = \Phi_I(0)\mathbf{e}_0 \cdot \mathbf{D}_0^{+2}(\boldsymbol{\kappa},\theta).\end{cases}$$

Obviously $\mathbf{e}_n \cdot \boldsymbol{\mathcal{D}}_{\pm+}\left(\hat{C}_{3\mathbf{k}}\boldsymbol{\kappa},\theta\right) = e^{i\frac{2}{3}(1-n)\pi}\mathbf{e}_n \cdot \boldsymbol{\mathcal{D}}_{\pm+}(\boldsymbol{\kappa},\theta)$. The other two cases with $\tau' = -1$, $\tau = -1$ or $\tau' = +1$, $\tau = -1$ can be obtained through time reversal relation, and the result is $\mathbf{e}_n \cdot \boldsymbol{\mathcal{D}}_{\pm-}\left(-\hat{C}_{3\mathbf{k}}\boldsymbol{\kappa},\theta\right) = e^{i\frac{2}{3}(-1-n)\pi}\mathbf{e}_n \cdot \boldsymbol{\mathcal{D}}_{\pm-}(-\boldsymbol{\kappa},\theta)$. So $\boldsymbol{\mathcal{D}}_{\tau'\tau}$ has the same rotational behavior as $\mathbf{D}_0^{2\tau}$, that is:

$$\mathbf{e}_n \cdot \boldsymbol{\mathcal{D}}_{\tau'\tau}\left(\hat{C}_{3\mathbf{k}}\mathbf{q},\theta\right) = e^{i\frac{2}{3}(\tau-n)\pi}\mathbf{e}_n \cdot \boldsymbol{\mathcal{D}}_{\tau'\tau}(\mathbf{q},\theta). \tag{S10}$$

**(2) In-plane mirror symmetry**

$\widehat{M}$ denotes the mirror reflection about the *yz* plane crossing a M-atom position $\mathbf{R}$, which changes $\mathbf{r} \equiv \left(r_x, r_y\right)$ to $\widehat{M}\mathbf{r} = \left(2R_x - r_x, r_y\right)$. $\widehat{M}_\mathbf{q}$ is the corresponding $\mathbf{k}$-space operation which changes $\mathbf{q} \equiv \left(q_x, q_y\right)$ to $\widehat{M}_\mathbf{q}\mathbf{q} = \left(-q_x, q_y\right)$. Since $\tau\mathbf{K} = \left(\tau\frac{4\pi}{3a}, 0\right)$, under mirror reflection, $\psi_{\tau,\mathbf{k}=0,\mathrm{c(v)}}\left(\widehat{M}\mathbf{r}\right) = \psi_{-\tau,\mathbf{k}=0,\mathrm{c(v)}}(\mathbf{r}) = \psi^*_{\tau,\mathbf{k}=0,\mathrm{c(v)}}(\mathbf{r})$ where the second step comes from time reversal symmetry. Together with Eq. (S1) one get $D_m\left(\widehat{M}\mathbf{r} - \mathbf{R}\right) = D_m\left(R_x - r_x, r_y - R_y\right) = \left(D_m(\mathbf{r} - \mathbf{R})\right)^*$. For $\theta = 0^\circ$ or $60^\circ$ the upper layer also has a *yz* mirror plane crossing $\mathbf{R}'$ so $D_{m'}\left(R'_x - r_x, r_y - R'_y\right) = \left(D_{m'}(\mathbf{r} - \mathbf{R}')\right)^*$. So

$$\begin{aligned} t_{m'}^{m}(\mathbf{q},\theta) &\equiv \iint \left(D_m(\mathbf{r}-\mathbf{R})\right)^* \widehat{H}_\mathrm{T} D_{m'}(\mathbf{r}-\mathbf{R}')\frac{e^{i\mathbf{q}\cdot(\mathbf{R}'-\mathbf{R})}}{\sqrt{\Omega'\Omega}} d\mathbf{r}d[\mathbf{R}'-\mathbf{R}] \\ &= \iint D_m\left(R_x - r_x, r_y - R_y\right)\widehat{H}_\mathrm{T}\left(D_{m'}\left(R'_x - r_x, r_y - R'_y\right)\right)^* \cdot \frac{e^{i\mathbf{q}\cdot(\mathbf{R}'-\mathbf{R})}d\mathbf{r}d[\mathbf{R}'-\mathbf{R}]}{\sqrt{\Omega'\Omega}} \\ &= \iint D_m(\mathbf{r}-\mathbf{R})\widehat{H}_\mathrm{T}\left(D_{m'}(\mathbf{r}-\mathbf{R}')\right)^* e^{i\left(\widehat{M}_\mathbf{q}\mathbf{q}\right)\cdot(\mathbf{R}'-\mathbf{R})}\frac{d\mathbf{r}d[\mathbf{R}'-\mathbf{R}]}{\sqrt{\Omega'\Omega}} \\ &= \left(t_{m'}^{m}\left(-\widehat{M}_\mathbf{q}\mathbf{q},\theta\right)\right)^* = \left(t_{m'}^{m}\left(q_x, -q_y, \theta\right)\right)^*. \end{aligned} \tag{S11}$$

Similarly

$$\mathbf{e}_\pm \cdot \mathbf{D}_0^{2\tau}(\mathbf{q},\theta) = -\left(\mathbf{e}_\pm \cdot \mathbf{D}_0^{2\tau}(q_x,-q_y,\theta)\right)^*. \tag{S12}$$

Therefore $t_{m'}^{m}(\mathbf{q},\theta)$ is real while $\mathbf{e}_\pm \cdot \mathbf{D}_0^{2\tau}(\mathbf{q},\theta)$ is pure imaginary when $q_y = 0$. On the other hand $\langle 0|\widehat{\mathbf{D}}|X_{\tau'(\tau)}\rangle$ is also pure imaginary, so $\mathbf{e}_\pm \cdot \boldsymbol{\mathcal{D}}_{\tau'\tau}(\mathbf{q},\theta)$ should be pure imaginary when $q_y = 0$. This result is exact only at $\theta = 0^\circ$ and $60^\circ$, as for other twisting angle the upper layer no longer has a *yz* mirror plane and $\mathbf{e}_\pm \cdot \boldsymbol{\mathcal{D}}_{\tau'\tau}(\mathbf{q},\theta)$ at $q_y = 0$ can have a real component in general. Nevertheless, for $\theta$ close to $0^\circ$ $(60^\circ)$, $t_{m'}^{m}(\mathbf{q},\theta) \approx t_{m'}^{m}(\mathbf{q},0^\circ)$ $(t_{m'}^{m}(\mathbf{q},\theta) \approx t_{m'}^{m}(\mathbf{q},60^\circ))$ and $\mathbf{D}_0^{2\tau}(\mathbf{q},\theta) \approx \mathbf{D}_0^{2\tau}(\mathbf{q},0^\circ)$ $(\mathbf{D}_0^{2\tau}(\mathbf{q},\theta) \approx \mathbf{D}_0^{2\tau}(\mathbf{q},60^\circ))$ are good approximations. Moreover, we note that the $\theta$ dependence comes from the fact that $D_{m,\mathbf{R}}$ only has $\hat{C}_3$-rotational symmetry instead of the continuous rotational symmetry. In the latter case (e.g. assuming $D_{m,\mathbf{R}}$ is just the *d*-orbitals of isolated atoms, as the leading order approximation), $t_{m'}^{m}$, $\mathbf{D}_0^{2\tau}$ and $\boldsymbol{\mathcal{D}}_{\tau'\tau}$ are independent of $\theta$.

## Supplementary Note III. Estimation of $\boldsymbol{\mathcal{D}}_{\tau'\tau}$ from *ab initio* calculations

Below, we give details on how $\boldsymbol{\mathcal{D}}_{\tau'\tau}(\tau\boldsymbol{\kappa})$ is estimated in the *ab inito* calculations of lattice matched commensurate MoSe2/WSe2 heterobilayers with $\theta = 0^\circ$ and $60^\circ$.

The momentum matrix element $\langle\psi_{\tau',\mathrm{c}}|\widehat{\mathbf{p}}|\psi_{\tau,\mathrm{v}}\rangle \equiv \langle\psi_{\tau',\mathbf{k}'=0,\mathrm{c}}|\widehat{\mathbf{p}}|\psi_{\tau,\mathbf{k}=0,\mathrm{v}}\rangle$ between the lowest conduction at $\tau'\mathbf{K}'$ and highest valence bands at $\tau\mathbf{K}$, predominantly in the MoSe2 layer and WSe2 layer respectively, can be directly obtained from the *ab initio* calculations. Its ratio to the interband momentum matrix element in a monolayer corresponds to (c.f. Eq. (S9)):

$$\frac{|\langle\psi_{\tau',\mathrm{c}}|\mathbf{e}_n \cdot \widehat{\mathbf{p}}|\psi_{\tau,\mathrm{v}}\rangle|}{|\langle\psi_{\tau,\mathrm{c}}|\widehat{\mathbf{p}}|\psi_{\tau,\mathrm{v}}\rangle|} \approx \left|\frac{\mathbf{e}_n \cdot \boldsymbol{\mathcal{D}}_{\tau'\tau,\mathbf{Q}=0}}{D}\right| = \left|\sum_n \sum_{\boldsymbol{\kappa}\in C_n} \mathbf{e}_n \cdot \frac{\boldsymbol{\mathcal{D}}_{\tau'\tau}(\tau\boldsymbol{\kappa})}{D} e^{-i\tau\boldsymbol{\kappa}\cdot\mathbf{r}_0}\right|, \tag{S13}$$

As discussed in the main text, we group the extended Dirac points $\tau\boldsymbol{\kappa}$ in the extended BZ scheme by concentric circles $C_n$. Since $\boldsymbol{\mathcal{D}}_{\tau'\tau}(\tau\boldsymbol{\kappa})$ is known to decay fast with the increase of $|\boldsymbol{\kappa}|$, we only keep three circles with the smallest radius ($C_0$, $C_1$ and $C_2$, see Supplementary Figure S3, and main text) in the summation. We use $\boldsymbol{\kappa}_j^{(l)}$ to dentoe the value of the $j$-th $\boldsymbol{\kappa}$ on $C_l$ circle (Supplementary Figure S3). The corresponding $\boldsymbol{\mathcal{D}}_{\tau'\tau}\left(\tau\boldsymbol{\kappa}_j^{(l)}\right)$ with different $j$ but fixed $l$ are related by symmetry properties given in Eq. (S10)-(S12), whose values are expressed as in Supplementary Figure S3 (a) and (b).

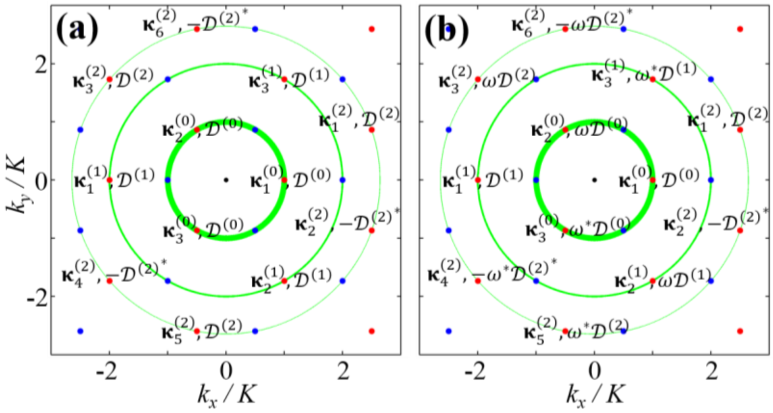


Supplementary Figure S3 | For $\tau = +1$, the different $\boldsymbol{\kappa}$ values (red dots) in the extended Brillouin zone

are markes as $\boldsymbol{\kappa}_j^{(l)}$ which denotes $j$-th $\boldsymbol{\kappa}$ on $C_l$ circle. The corresponding $\boldsymbol{\mathcal{D}}_{\tau'+}\left(\boldsymbol{\kappa}_j^{(l)}\right)$ values are related by symmetry properties, as illustrated for (a) $\mathcal{D} \equiv \mathbf{e}_+ \cdot \boldsymbol{\mathcal{D}}_{\tau'+}$. (b) $\mathcal{D} \equiv \mathbf{e}_- \cdot \boldsymbol{\mathcal{D}}_{\tau'+}$.

Note that $D$ is pure imaginary so $-(\mathbf{e}_n \cdot \boldsymbol{\mathcal{D}}_{\tau'\tau})^*/D = (\mathbf{e}_n \cdot \boldsymbol{\mathcal{D}}_{\tau'\tau}/D)^*$. Eq. (S13) becomes:

$$\left| f^{(0)}(\mathbf{r}_0)\mathbf{e}_n \cdot \frac{\boldsymbol{\mathcal{D}}_{\tau'\tau}^{(0)}}{D} + f^{(1)}(\mathbf{r}_0)\mathbf{e}_n \cdot \frac{\boldsymbol{\mathcal{D}}_{\tau'\tau}^{(1)}}{D} + f_1^{(2)}(\mathbf{r}_0)\mathbf{e}_n \cdot \frac{\boldsymbol{\mathcal{D}}_{\tau'\tau}^{(2)}}{D} + f_2^{(2)}(\mathbf{r}_0)\left(\mathbf{e}_n \cdot \frac{\boldsymbol{\mathcal{D}}_{\tau'\tau}^{(2)}}{D}\right)^* \right|. \qquad \text{(S14)}$$

where $\boldsymbol{\mathcal{D}}_{\tau'\tau}^{(l)} \equiv \boldsymbol{\mathcal{D}}_{\tau'\tau}\left(\tau\boldsymbol{\kappa}_1^{(l)}\right)$. The coefficient $f$ depends on $\mathbf{r}_0$. For $\mathbf{e}_\tau \cdot \boldsymbol{\mathcal{D}}_{\tau'\tau}/D$,

$$f^{(0)}(\mathbf{r}_0) \equiv e^{-i\tau\boldsymbol{\kappa}_1^{(0)}\cdot\mathbf{r}_0} + e^{-i\tau\boldsymbol{\kappa}_2^{(0)}\cdot\mathbf{r}_0} + e^{-i\tau\boldsymbol{\kappa}_3^{(0)}\cdot\mathbf{r}_0}, f^{(1)}(\mathbf{r}_0) \equiv e^{-i\tau\boldsymbol{\kappa}_1^{(1)}\cdot\mathbf{r}_0} + e^{-i\tau\boldsymbol{\kappa}_2^{(1)}\cdot\mathbf{r}_0} + e^{-i\tau\boldsymbol{\kappa}_3^{(1)}\cdot\mathbf{r}_0}$$

$$f_1^{(2)}(\mathbf{r}_0) \equiv e^{-i\tau\boldsymbol{\kappa}_1^{(2)}\cdot\mathbf{r}_0} + e^{-i\tau\boldsymbol{\kappa}_3^{(2)}\cdot\mathbf{r}_0} + e^{-i\tau\boldsymbol{\kappa}_5^{(2)}\cdot\mathbf{r}_0}, f_2^{(2)}(\mathbf{r}_0) \equiv e^{-i\tau\boldsymbol{\kappa}_2^{(2)}\cdot\mathbf{r}_0} + e^{-i\tau\boldsymbol{\kappa}_4^{(2)}\cdot\mathbf{r}_0} + e^{-i\tau\boldsymbol{\kappa}_6^{(2)}\cdot\mathbf{r}_0}$$

While for $\mathbf{e}_{-\tau} \cdot \boldsymbol{\mathcal{D}}_{\tau'\tau}/D$:

$$f^{(0)}(\mathbf{r}_0) \equiv e^{-i\tau\boldsymbol{\kappa}_1^{(0)}\cdot\mathbf{r}_0} + \omega e^{-i\tau\boldsymbol{\kappa}_2^{(0)}\cdot\mathbf{r}_0} + \omega^* e^{-i\tau\boldsymbol{\kappa}_3^{(0)}\cdot\mathbf{r}_0},$$

$$f^{(1)}(\mathbf{r}_0) \equiv e^{-i\tau\boldsymbol{\kappa}_1^{(1)}\cdot\mathbf{r}_0} + \omega e^{-i\tau\boldsymbol{\kappa}_2^{(1)}\cdot\mathbf{r}_0} + \omega^* e^{-i\tau\boldsymbol{\kappa}_3^{(1)}\cdot\mathbf{r}_0},$$

$$f_1^{(2)}(\mathbf{r}_0) \equiv e^{-i\tau\boldsymbol{\kappa}_1^{(2)}\cdot\mathbf{r}_0} + \omega e^{-i\tau\boldsymbol{\kappa}_3^{(2)}\cdot\mathbf{r}_0} + \omega^* e^{-i\tau\boldsymbol{\kappa}_5^{(2)}\cdot\mathbf{r}_0},$$

$$f_2^{(2)}(\mathbf{r}_0) \equiv e^{-i\tau\boldsymbol{\kappa}_2^{(2)}\cdot\mathbf{r}_0} + \omega^* e^{-i\tau\boldsymbol{\kappa}_4^{(2)}\cdot\mathbf{r}_0} + \omega e^{-i\tau\boldsymbol{\kappa}_6^{(2)}\cdot\mathbf{r}_0},$$

where $\omega \equiv e^{-i\tau\frac{2}{3}\pi}$.

Note that $\mathbf{e}_\pm \cdot \boldsymbol{\mathcal{D}}_{\tau'\tau}^{(0)}/D$ and $\mathbf{e}_\pm \cdot \boldsymbol{\mathcal{D}}_{\tau'\tau}^{(1)}/D$ are real, while $\mathbf{e}_\pm \cdot \boldsymbol{\mathcal{D}}_{\tau'\tau}^{(2)}/D$ can be complex. We choose four heterobilayer configurations with different values for the layer translation $\mathbf{r}_0$ and find $\langle\psi_{\tau',\mathrm{c}}|\hat{\mathbf{p}}|\psi_{\tau,\mathrm{v}}\rangle$ from *ab initio* calculation. $\boldsymbol{\mathcal{D}}_{\tau'\tau}$ can then be solved from Eq. (S14).

The *ab initio* calculations for the $MoSe_2/WSe_2$ heterobilayer are performed with the plane waves and the projector-augumented wave (PAW) method implemented in the Quantum Espresso package [11]. The Perdew-Burke-Ernzerhof (PBE) exchange-correlation functional [12] is used for all the calculations. The band structure for all the heterobilayer structures are calculated with the scalar relativistic pseudopotential without including the spin-orbit coupling, and the energy cutoff is chosen as 60 Ry for all the structures. A $15 \times 15 \times 1$ Monkhorst-Pack $\mathbf{k}$-point mesh is used to sample the Brillouin zone, and the convergence criterion for total energy is $10^{-10}$ Ry in each electronic self-consistent calculations. The structure parameters are taken from Ref. [13]. For both $\theta = 0^\circ$ and $60^\circ$, the heterobilayer interlayer distance is set as the average of the homobilayer $MoSe_2$ and $WSe_2$ AA- and AB-stacking value: $d = (d_{\mathrm{Mo,AA}} + d_{\mathrm{Mo,AB}} + d_{\mathrm{W,AA}} + d_{\mathrm{W,AB}})/4 = 3.575$ Å, but the interlayer translation $\mathbf{r}_0$ can be various different values. The obtained results are shown in Table 1.

| | $\lvert \mathbf{e}_\tau \cdot \boldsymbol{\mathcal{D}}_{\tau'\tau}/D \rvert$ | | | $\lvert \mathbf{e}_{-\tau} \cdot \boldsymbol{\mathcal{D}}_{\tau'\tau}/D \rvert$ | | | $\lvert \mathbf{e}_0 \cdot \boldsymbol{\mathcal{D}}_{\tau'\tau}/D \rvert$ |
|---|---|---|---|---|---|---|---|
| | $C_0$ | $C_1$ | $C_2$ | $C_0$ | $C_1$ | $C_2$ | $C_0$ |
| $\theta = 0^\circ$ | 0.051 | 0.001 | 0.001 | 0.011 | $5\times10^{-4}$ | $5\times10^{-5}$ | 0.009 |
| $\theta = 60^\circ$ | 0.010 | 0.001 | $5\times10^{-5}$ | 0.051 | 0.001 | $5\times10^{-4}$ | 0.009 |

Table 1. The obtained $\lvert \mathbf{e}_\pm \cdot \boldsymbol{\mathcal{D}}_{\tau'\tau}/D \rvert$ on $C_0$, $C_1$ and $C_2$ for $\theta = 0^\circ$ and $\theta = 60^\circ$ $MoSe_2/WSe_2$ heterobilayers from *ab initio* calculation. For completeness the out-of-plane ($\mathbf{e}_0 \equiv \mathbf{z}$) component on $C_0$ is also given.

The corresponding photon polarization can be written in the Bloch sphere representation: $\cos\alpha\,\hat{\sigma}_+ + \mathrm{e}^{i\varphi}\sin\alpha\,\hat{\sigma}_-$. The elliptical polarization major to minor axis ratio is given by $\frac{\cos\alpha+\sin\alpha}{|\cos\alpha-\sin\alpha|}$. The ellipticity (flattening) is defined as $\epsilon \equiv 1 - \frac{|\cos\alpha-\sin\alpha|}{\cos\alpha+\sin\alpha}$, which reaches its maximum value 1 (minimum value 0) for the linear (circular) polarized case. For the heterobilayer $MoSe_2/WSe_2$, we find the axis ratio $\frac{\cos\alpha+\sin\alpha}{|\cos\alpha-\sin\alpha|}\sim 1.55$ ($\sim$1.49) and ellipticity $\epsilon\sim 0.33$ ($\sim$0.35) for $\theta$ near $60^\circ$ ($0^\circ$).

We analyze the accuracy of the above *ab initio* results. The error in the *ab initio* calculation of interlayer transition dipole in lattice-matching bilayer can be determined at the configuration with the interlayer translation $\mathbf{r}_0 = 2(\mathbf{a}_1 + \mathbf{a}_2)/3$, where the 3-fold rotational symmetry dictates the in-plane component of interlayer dipole matrix element to be exactly zero. The value given from the *ab initio* calculation is indeed a number extremely close to zero, at least four orders of magnitude smaller than $D$ ($D$ being the transition dipole of intralayer exciton). This could be taken as the error bar for the *ab initio* calculation, which is two to three orders smaller compared with the extracted interlayer transition dipole of $\sim 0.05D$ at general twisting angle.

Besides, symmetry analysis has dictated the $\mathbf{r}_0$-dependence of the in-plane component of interlayer dipole to be (see Eq. (5) in the maintext):

$$\boldsymbol{\mathcal{D}}_{\tau'\tau}(\mathbf{r}_0) = \left(e^{-i\tau\mathbf{K}\cdot\mathbf{r}_0} + e^{-i\tau\hat{C}_3\mathbf{K}\cdot\mathbf{r}_0} + e^{-i\tau\hat{C}_3^2\mathbf{K}\cdot\mathbf{r}_0}\right)D_1\mathbf{e}_\tau + \left(e^{-i\tau\mathbf{K}\cdot\mathbf{r}_0} + e^{-i\tau\left(\hat{C}_3\mathbf{K}\cdot\mathbf{r}_0+\frac{2\pi}{3}\right)} + e^{-i\tau\left(\hat{C}_3^2\mathbf{K}\cdot\mathbf{r}_0+\frac{4\pi}{3}\right)}\right)D_2\mathbf{e}_{-\tau}, \quad \text{(S15)}$$

where $D_{1,2}$ are two complex numbers independent of $\mathbf{r}_0$. This symmetry dictated form can be compared with the $\mathbf{r}_0$-dependence of the interlayer dipole directly from *ab initio* calculation. The agreement between the two can be another measure of the error in the *ab initio* calculation. The comparison is given in Supplementary Figure S4, which shows perfect agreement.

Based on these analysis, we conclude that the numerical accuracy of the calculation to be good.

At last, we would like to note that the magnitude of the interlayer coupling depends on the layer separation. The layer separation values $d_{\mathrm{Mo,AA}}$, $d_{\mathrm{Mo,AB}}$, $d_{\mathrm{W,AA}}$ and $d_{\mathrm{W,AB}}$ used here are taken from Ref. [13], where the calculation uses PBE+vdW functionals. There can be other possible values for the layer separations (e.g. calculated under structural relaxation in different approximations, with or without vdW correction). Nevertheless, within the reasonable range of values for the layer separation, the interlayer coupling is found to be always weak compared to the band offsets [14], so the perturbative approach (Eq. (S5)) remains valid. The choice of layer separation can change the overall strength of the interlayer exciton dipole, but not affecting the

qualitative features of the light coupling properties (i.e. the location and elliptical polarization of light cones at finite twisting, and translation dependence of polarization and dipole strength at AA-like and AB-like stacking).

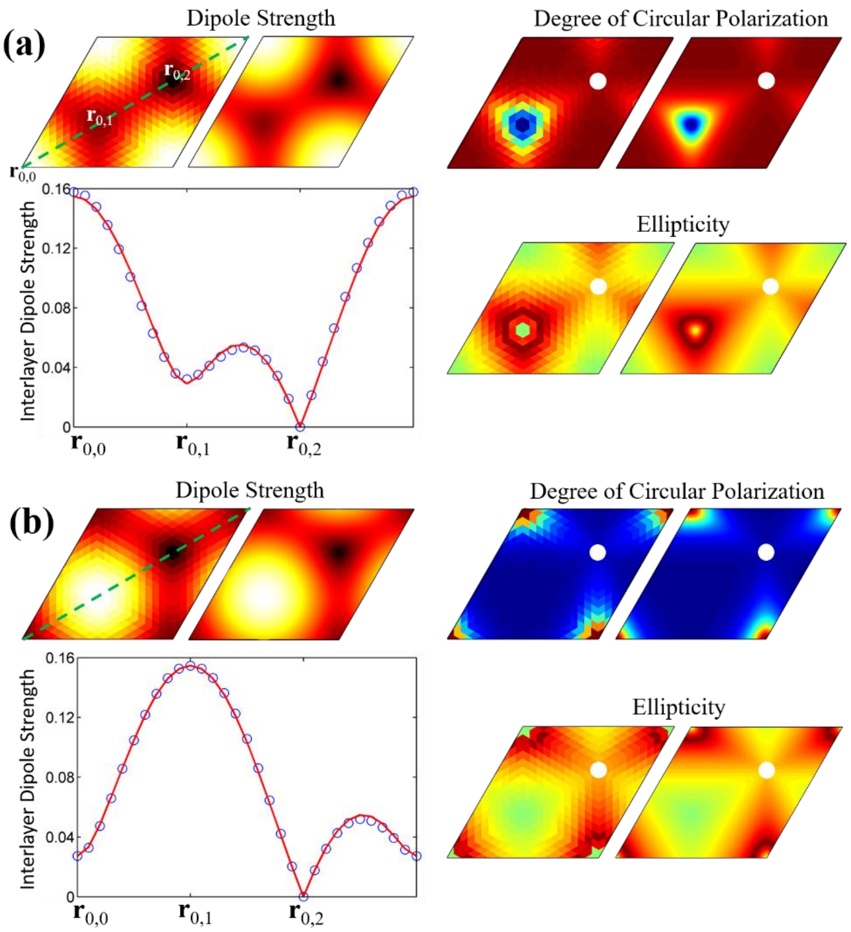


Supplementary Figure S4 | Comparison between *ab initio* calculated $\boldsymbol{\mathcal{D}}_{\tau'\tau}(\mathbf{r}_0)$ and its symmetry dictated form. (a) For $\boldsymbol{\mathcal{D}}_{++}(\mathbf{r_0})$ at $\theta = 0^{\circ}$, and (b) for $\boldsymbol{\mathcal{D}}_{-+}(\mathbf{r_0})$ at $\theta = 60^{\circ}$. In the surface plots, for each group of comparison for the dipole strength and polarization, the left panel is the *ab initio* result, and the right panel is the plot using the symmetry dictated form in Eq. (S15). The 2D plot of the dipole strength is a line cut along the dashed green line, where the symbols are the *ab initio* results and the red curve is the symmetry dictated function.

## Supplementary Note IV. Band-to-band absorption edge

Consider an unbound electron-hole pair $|e_{\tau',\mathbf{k}'}\rangle|h_{\tau,\mathbf{k}}\rangle$. By the same argument based on Fourier expansion of the Bloch functions, the electron-hole pair can recombine only when $\mathbf{k}' + \tau'\mathbf{K}' + \mathbf{G}' = -\mathbf{k} + \tau\mathbf{K} + \mathbf{G}$. The Umklapp-type processes with finite $\mathbf{G}'$ and $\mathbf{G}'$ are very weak, so we focus on the case $\mathbf{G}' = 0$ and $\mathbf{G} = 0$. Such an electron-hole pair has an energy $\frac{\hbar^2 Q^2}{2M_0} + \frac{\hbar^2 q^2}{2\mu} + \Delta_g$ with $\mathbf{Q} \equiv \mathbf{k}' + \mathbf{k} = \tau\mathbf{K} - \tau'\mathbf{K}'$, $\mathbf{q} \equiv (m_h\mathbf{k}' - m_e\mathbf{k})/M_0$ and $\mu \equiv m_e m_h/M_0$. Summing over all such bright electron-hole pairs, the optical oscillator strength at a given energy

$E$ is proportional to

$$E\sum_{\mathbf{Q},\mathbf{q}}\delta\left(E-\frac{\hbar^2Q^2}{2M_0}-\frac{\hbar^2q^2}{2\mu}-\Delta_g\right)\delta_{\mathbf{Q},\tau\mathbf{K}-\tau'\mathbf{K}'}\left|\mathbf{d}_{\mathbf{k}'+\tau'\mathbf{K}',-\mathbf{k}+\tau\mathbf{K}}\right|^2$$

$$\approx E|\mathbf{d}_{\mathrm{cv}}|^2\sum_{\mathbf{Q},\mathbf{q}}\delta\left(E-\frac{\hbar^2Q^2}{2M_0}-\frac{\hbar^2q^2}{2\mu}-\Delta_g\right)\delta_{\mathbf{Q},\tau\mathbf{K}-\tau'\mathbf{K}'}$$

$$\propto E|\mathbf{d}_{\mathrm{cv}}|^2\Theta\left(E-\frac{\hbar^2|\tau\mathbf{K}-\tau'\mathbf{K}'|^2}{2M_0}-\Delta_g\right).$$

Here $\Theta$ is the Heaviside step function. In the first step we have used a leading order approximation $\left|\mathbf{d}_{\mathbf{k}'+\tau'\mathbf{K}',-\mathbf{k}+\tau\mathbf{K}}\right|^2\approx|\mathbf{d}_{\mathrm{cv}}|^2$ for the band-to-band transition dipole. So the absorption edge for the interlayer band-to-band transition in the heterobilayers is at $\frac{\hbar^2|\tau\mathbf{K}-\tau'\mathbf{K}'|^2}{2M_0}+\Delta_g$. In comparison, the energy of the six-fold degenerate main light cones is $\frac{\hbar^2|\tau\mathbf{K}-\tau'\mathbf{K}'|^2}{2M_0}+\Delta_g-E_b$, separated from the band-to-band absorption edge by the binding energy $E_b$.


[1] H. Yu, G.-B. Liu, P. Gong, X. Xu, and W. Yao, Nat. Commun. **5**, 3876 (2014).

[2] F. Bassani and G. P. Parravicini, *Electronic states and optical transitions in solids* (Pergamon Press, 1975).

[3] S. A. Moskalenko and D. W. Snoke, *Bose-Einstein Condensation of Excitons and Biexcitons* (Cambridge University Press, 2000).

[4] D. Y. Qiu, F. H. d. Jornada, and S. G. Louie, Phys. Rev. Lett. **111**, 216805 (2013).

[5] T. C. Berkelbach, M. S. Hybertsen, and D. R. Reichman, Phys. Rev. B **88**, 045318 (2013).

[6] P. Rivera *et al.*, Nat. Commun. **6**, 6242 (2015).

[7] M.-H. Chiu *et al.*, Nat. Commun. **6**, 7666 (2015).

[8] M.-H. Chiu, M.-Y. Li, W. Zhang, W.-T. Hsu, W.-H. Chang, M. Terrones, H. Terrones, and L.-J. Li, ACS Nano **8**, 9649 (2014).

[9] S. Dufferwiel *et al.*, arXiv:1505.04438 (2015).

[10] R. Bistritzer and A. H. MacDonald, Phys. Rev. B **81**, 245412 (2010).

[11] P. Giannozzi *et al.*, J. Phys. Condens. Matter **21**, 395502 (2009).

[12] J. P. Perdew, K. Burke, and M. Ernzerhof, Phys. Rev. Lett. **77**, 3865 (1996).

[13] S. Bhattacharyya and A. K. Singh, Phys. Rev. B **86**, 075454 (2012).

[14] K. Liu *et al.*, Nat. Commun. **5**, 4966 (2014).
